# Supplementary material for: DriveStack-VLA: Render-Teacher Alignment for BEV-Based DeepStack Vision-Language-Action Model
Source: arXiv:2606.24051 source file (2026-06-23)
Supplement: Supplementary file 3 [file fig4_select_vis3.tex]

\begin{figure*}[t]
      \centering
       % 1. 压减图片与 Caption 之间的距离
      \setlength{\abovecaptionskip}{2pt} 
      % 2. 压减 Caption 与下方正文之间的距离
      \setlength{\belowcaptionskip}{-18pt}
      \includegraphics[width=\linewidth]{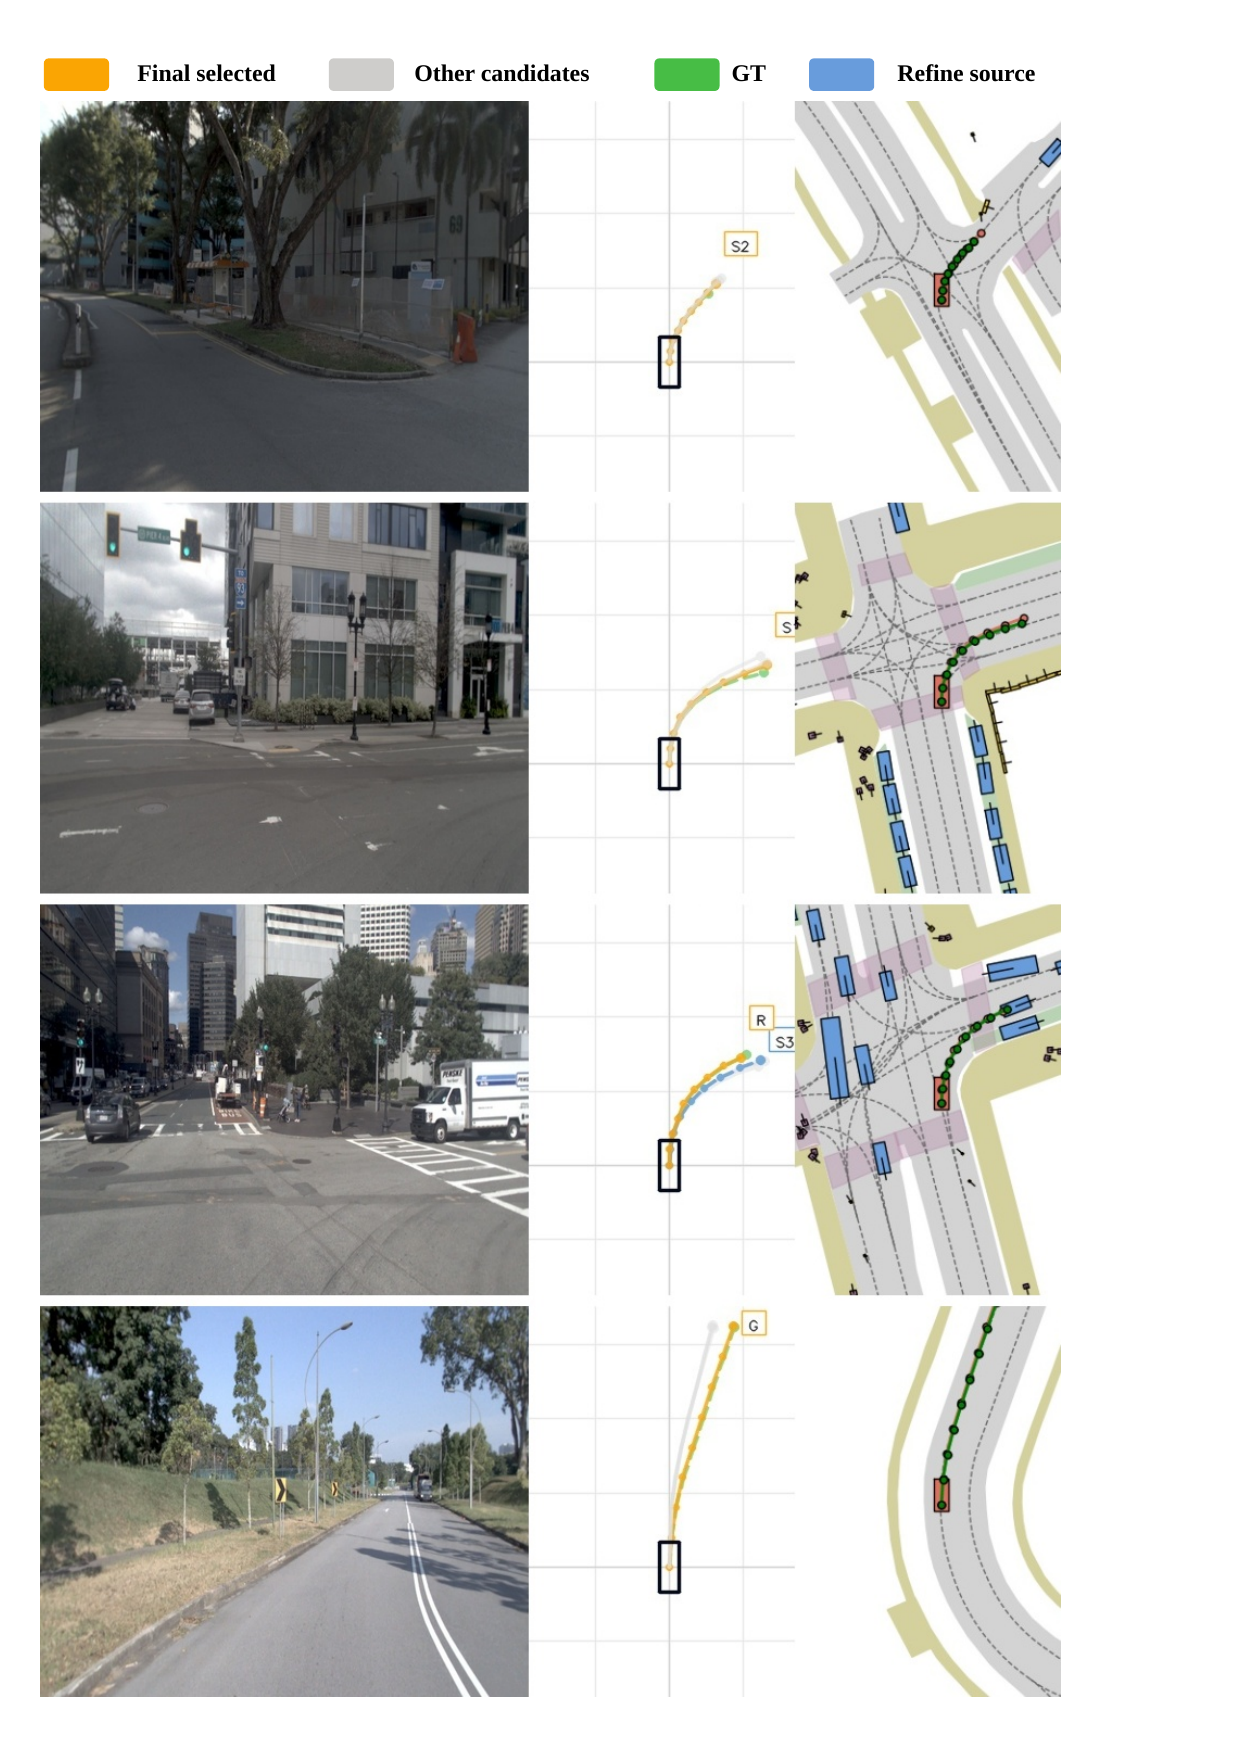}
      % \vspace{-1pt}
      \captionsetup{font={small}}
      \caption{Qualitative results on the Navtest benchmark for the turn right scenario.
      }
      \label{fig:select_vis3}
      % \vspace{-2pt} 
\end{figure*}
