# Supplementary material for: DriveStack-VLA: Render-Teacher Alignment for BEV-Based DeepStack Vision-Language-Action Model
Source: arXiv:2606.24051 source file (2026-06-23)
Supplement: Supplementary file 4 [file A_additional_related_works.tex]

% \section{Additional Related Works}
% \label{sec:addtional_related_works}

% \subsection{Rendering for autonomous driving.}
% Synthetic view generation is a common approach for augmenting recovery data beyond the logged trajectory. Neural rendering methods, such as NeRF \cite{mildenhall2021nerf} and Gaussian Splatting \cite{kerbl20233d}, can replay scenes with high visual fidelity, but these methods remain slow and difficult to scale. 
% RAP \cite{feng2025rap} demonstrates that lightweight 3D rasterization can generate controllable views that emphasize lanes, agents, and signals, and that it aligns raster features with real-image features in a shared feature space.
% % For VLA driving models, the primary supervision signal includes not only image features, but also the attention patterns between action tokens and visual tokens in the LLM decoder. 
% In this work, we treat rasterized images as a teacher modality and transfer supervision to real images via masked camera-token alignment and action-to-vision attention distillation \cite{zagoruyko2016paying}. 
% This design provides a direct and efficient way to couple raster augmentation with planning, encouraging the LLM decoder
% to attend to safety-critical cues during planning.
